# Supplementary material for: Incremental Concept Learning via Online Generative Memory Recall
Source: arXiv:1907.02788 source file (2019-07-05)
Supplement: Supplementary file 1 [file appendix.tex]

% use section* for acknowledgment
\section*{Acknowledgment}
The authors would like to thank...

Appendix one text goes here.
\appendices
\section{Proof of the First Zonklar Equation}
Appendix one text goes here.

% you can choose not to have a title for an appendix
% if you want by leaving the argument blank
\section{}
Appendix two text goes here.
